# Supplementary material for: Bayesian Hierarchical Spatial Regression Models for Spatial Data in the Presence of Missing Covariates with Applications
Source: arXiv:2007.02228 source file (2020-07-05)
Supplement: Supplementary file 1 [file supplementary-2.pdf]

# Supplementary Materials: Additional Figure and Tables for Bayesian Hierarchical Spatial Regression Models for Spatial Data in the Presence of Missing Covariates with Applications

Zhihua Ma[*†], Guanyu Hu[†], and Ming-Hui Chen[†],
[*]Department of Statistics, Shenzhen University, Shenzhen, China
[†]Department of Statistics, University of Connecticut, Storrs, CT, USA

April 5, 2020

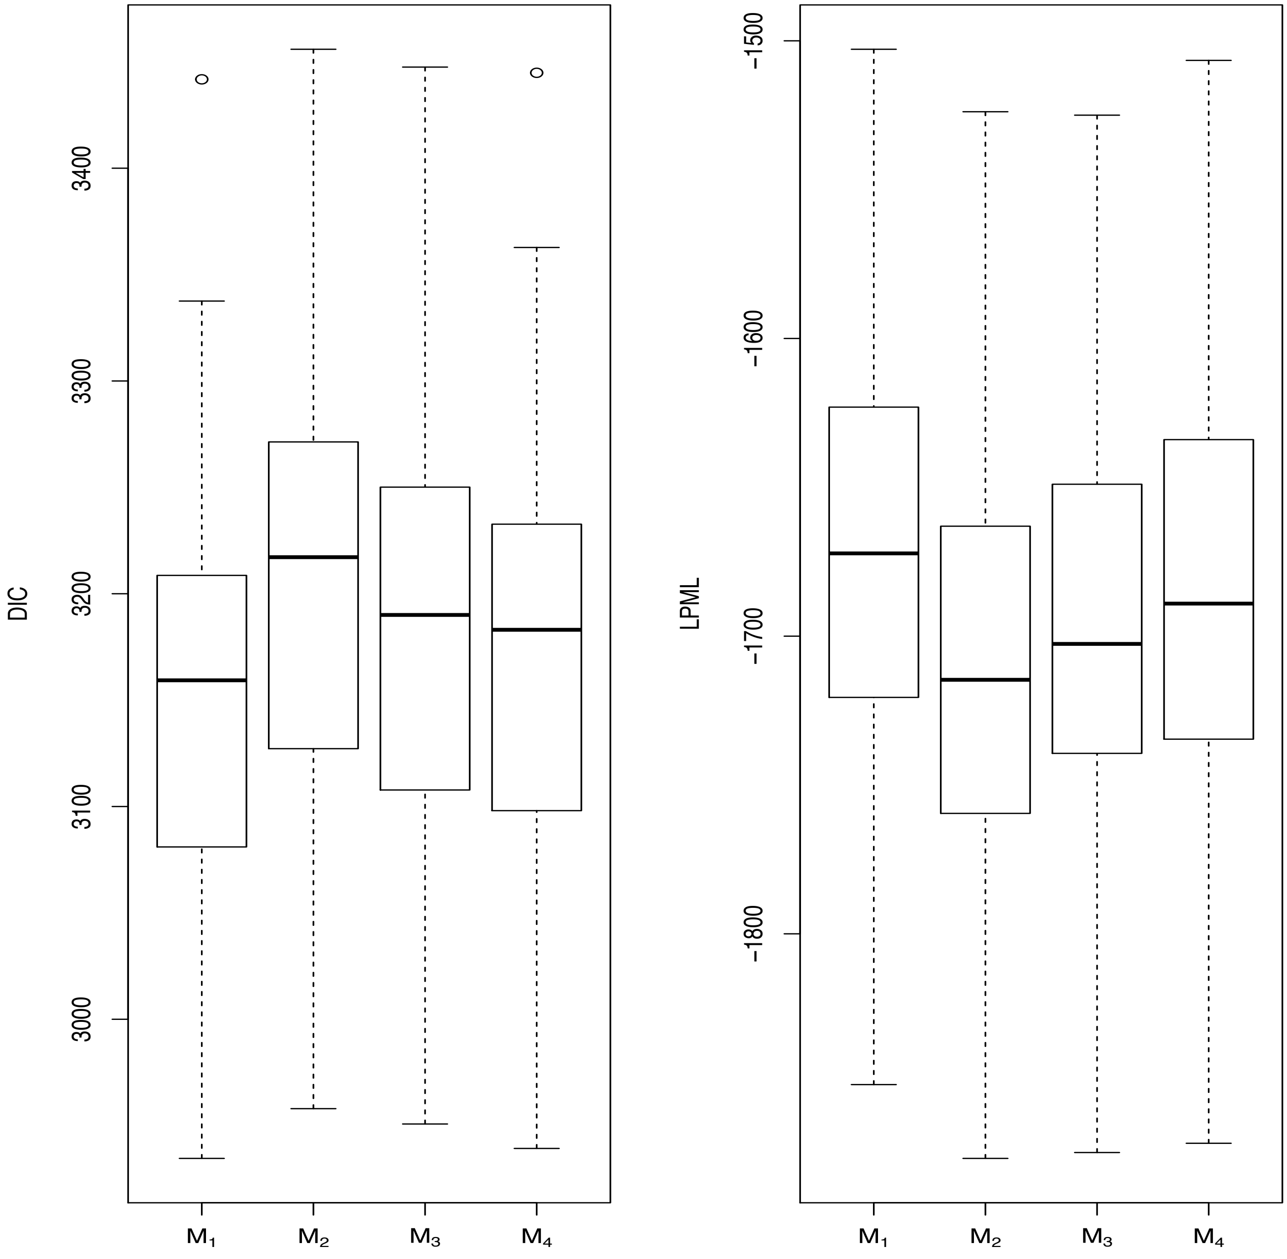


Figure S1: mDIC and mLPML values for models $M_1$, $M_2$, $M_3$ and $M_4$ in the simulation study

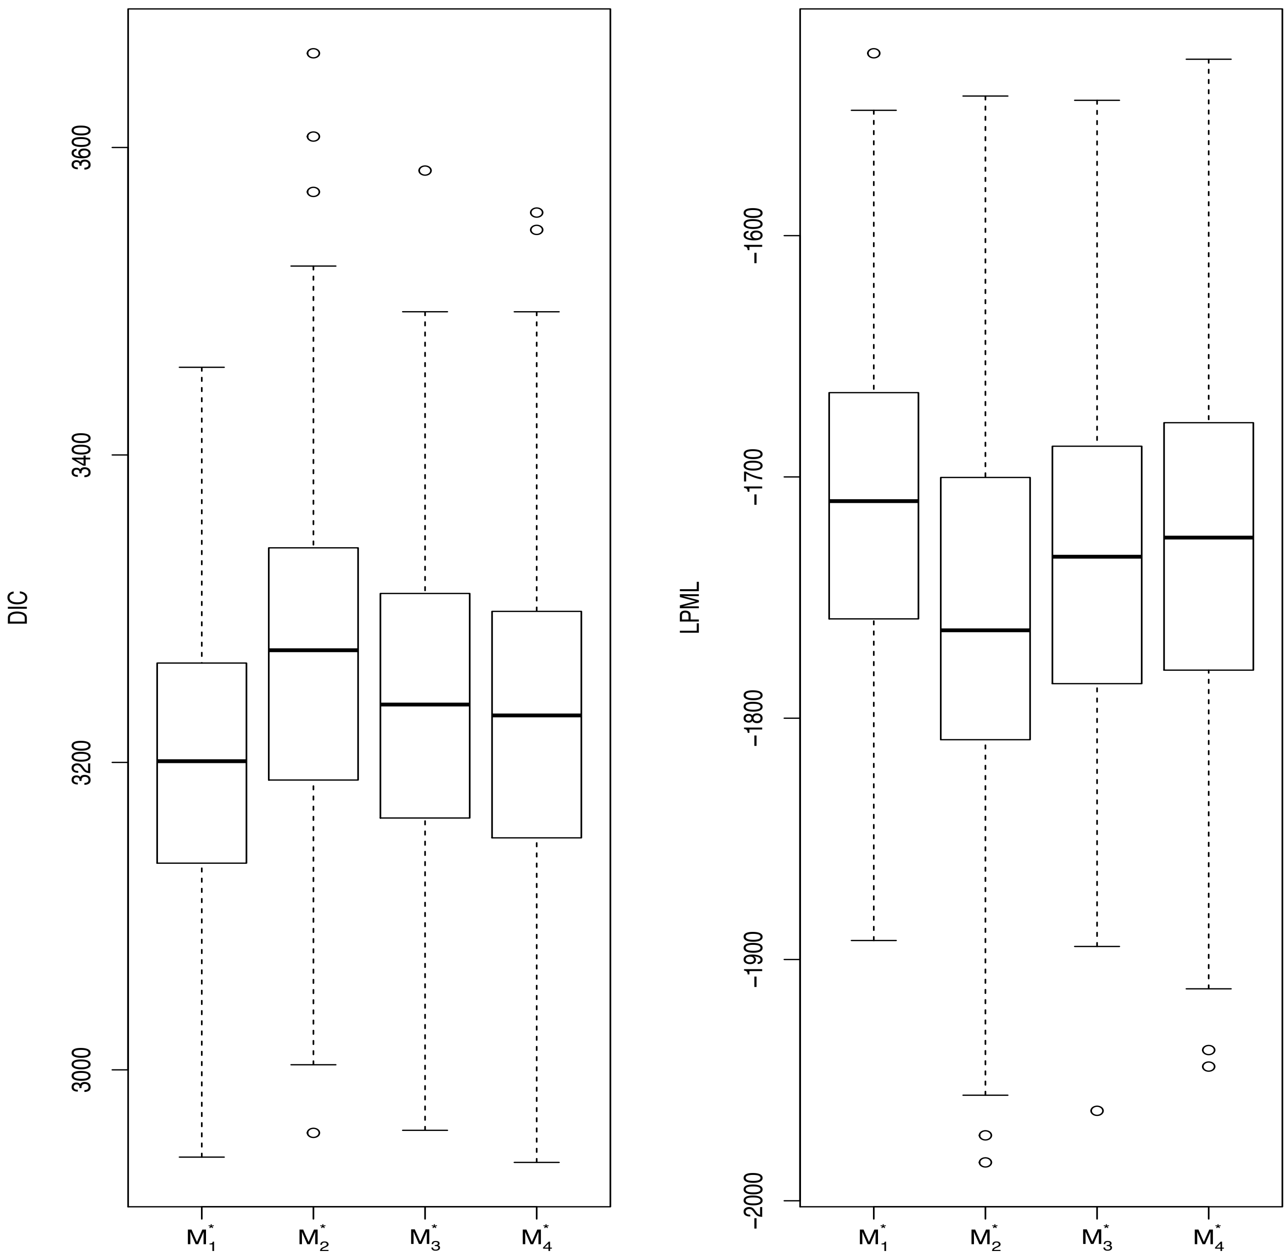


Figure S2: mDIC and mLPML values for models $M_1^*$, $M_2^*$, $M_3^*$ and $M_4^*$ in the simulation study

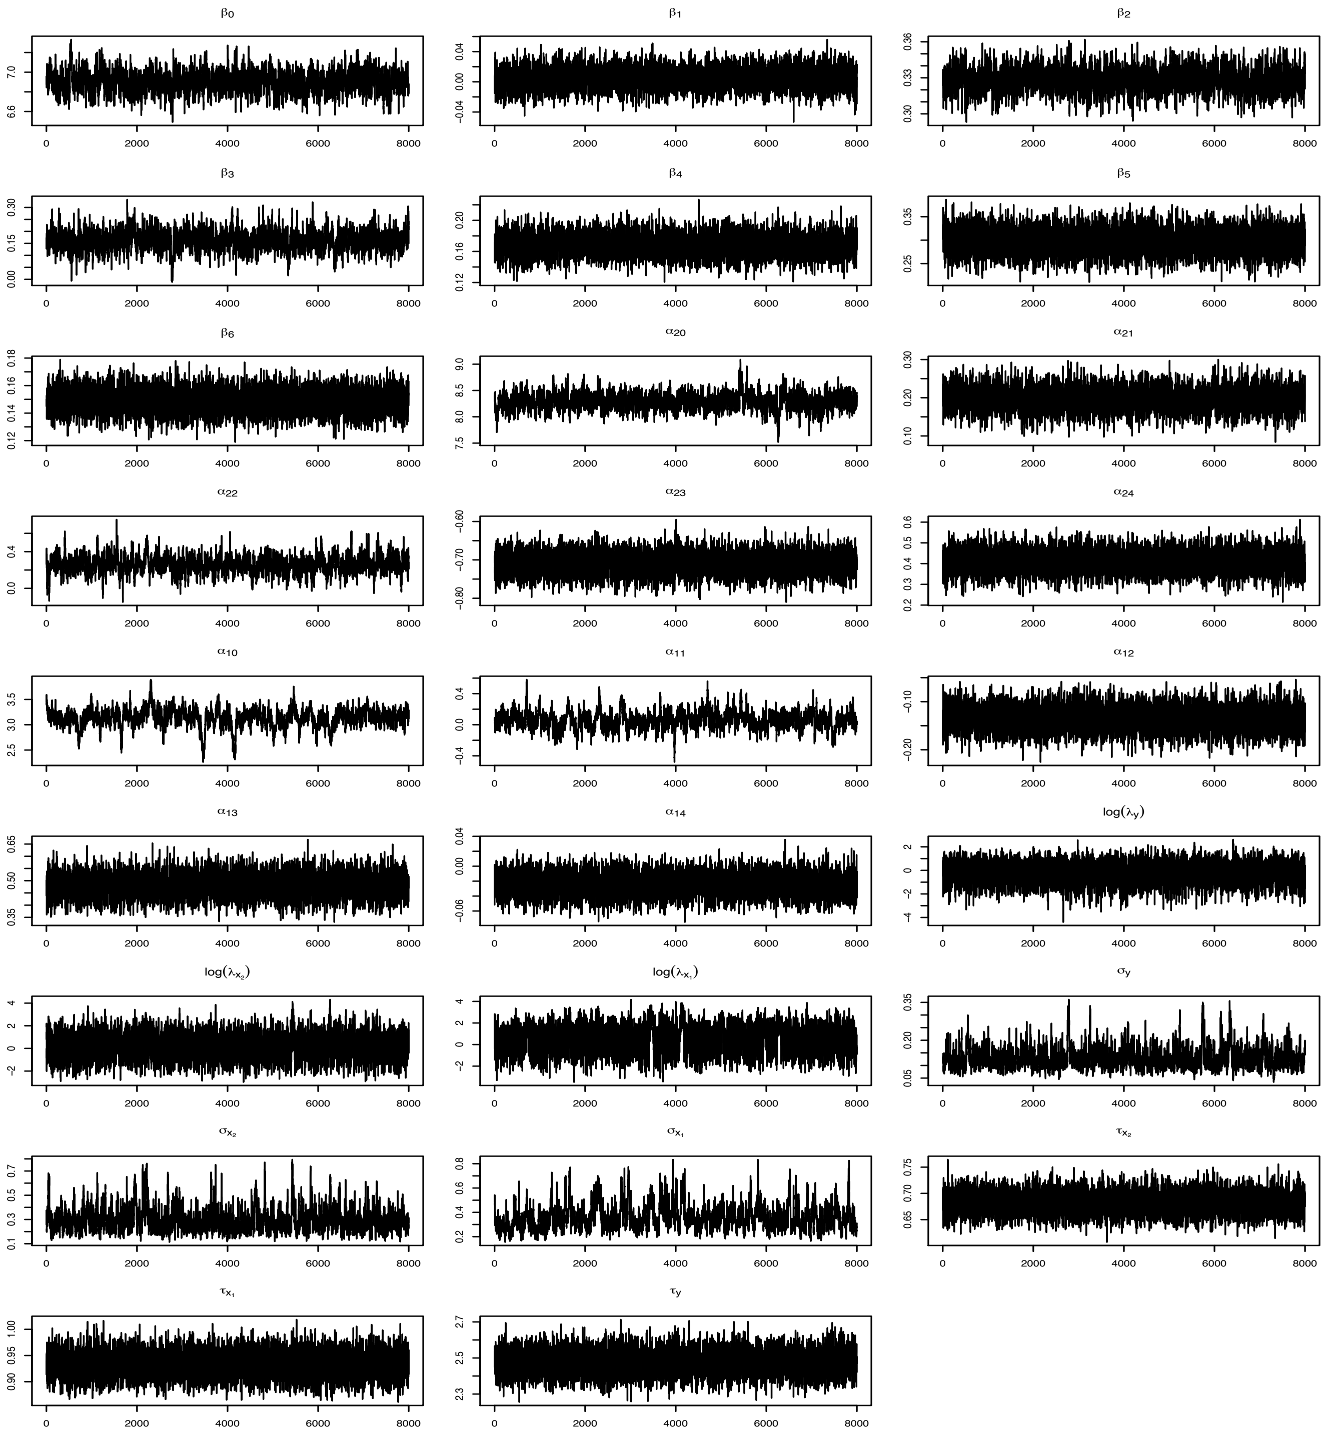


Figure S3: Trace plots of parameters under $M_1^{real}$

Table S1: Simulation results of posterior estimates of parameters in the spatial response model with missing covariate models $M_2$, $M_3$, and $M_4$

| | True value | $M_2$ | | | | $M_3$ | | | |
|---|---|---|---|---|---|---|---|---|---|
| | | Bias | SD | MSE | CP | Bias | SD | MSE | CP |
| $\beta_0$ | 1 | -0.0090 | 0.5071 | 0.2573 | 0.92 | 0.0322 | 0.5044 | 0.2554 | 0.94 |
| $\beta_1$ | 1.5 | 0.0818 | 0.1177 | 0.0205 | 0.74 | 0.1266 | 0.1089 | 0.0279 | 0.71 |
| $\beta_2$ | 1 | -0.0571 | 0.0531 | 0.0061 | 0.64 | -0.0598 | 0.0499 | 0.0061 | 0.66 |
| $\beta_3$ | 2 | 0.0478 | 0.0677 | 0.0069 | 0.85 | -0.0023 | 0.0655 | 0.0043 | 0.91 |
| $\tau_y$ | 1 | -0.0219 | 0.0636 | 0.0045 | 0.91 | -0.0047 | 0.0663 | 0.0044 | 0.89 |

| | True value | $M_4$ | | | |
|---|---|---|---|---|---|
| | | Bias | SD | MSE | CP |
| $\beta_0$ | 1 | -0.0642 | 0.5133 | 0.2676 | 0.92 |
| $\beta_1$ | 1.5 | -0.0675 | 0.1029 | 0.0152 | 0.86 |
| $\beta_2$ | 1 | 0.0170 | 0.0482 | 0.0026 | 0.88 |
| $\beta_3$ | 2 | 0.0425 | 0.0628 | 0.0058 | 0.83 |
| $\tau_y$ | 1 | -0.0092 | 0.0631 | 0.0041 | 0.91 |

Table S2: Simulation results of posterior estimates of parameters in the spatial response model with missing covariate models $M_2^*$, $M_3^*$, and $M_4^*$

| | True value | $M_2^*$ | | | | $M_3^*$ | | | |
|---|---|---|---|---|---|---|---|---|---|
| | | Bias | SD | MSE | CP | Bias | SD | MSE | CP |
| $\beta_0$ | 1 | -0.0051 | 0.6632 | 0.2701 | 0.97 | 0.1001 | 0.6016 | 0.2774 | 0.94 |
| $\beta_1$ | 1.50 | 0.0805 | 0.0952 | 0.0213 | 0.79 | 0.1457 | 0.0943 | 0.0334 | 0.66 |
| $\beta_2$ | 1 | -0.0676 | 0.0427 | 0.0077 | 0.63 | -0.0729 | 0.0420 | 0.0077 | 0.63 |
| $\beta_3$ | 2 | 0.0786 | 0.0599 | 0.0097 | 0.74 | 0.0113 | 0.0584 | 0.0026 | 0.98 |
| $\sigma_y$ | 1.41 | 0.2668 | 0.3978 | 0.2079 | 0.87 | 0.1754 | 0.3809 | 0.1189 | 0.95 |
| $\log(\lambda_y)$ | 1.10 | -0.6149 | 0.9333 | 0.7752 | 0.98 | -0.6122 | 0.9227 | 0.7894 | 0.98 |
| $\tau_y$ | 1 | -0.0441 | 0.0605 | 0.0067 | 0.85 | -0.0180 | 0.0609 | 0.0043 | 0.91 |

| | True value | $M_4^*$ | | | |
|---|---|---|---|---|---|
| | | Bias | SD | MSE | CP |
| $\beta_0$ | 1 | 0.0194 | 0.6185 | 0.2637 | 0.96 |
| $\beta_1$ | 1.5 | -0.0971 | 0.0932 | 0.0228 | 0.85 |
| $\beta_2$ | 1 | 0.0225 | 0.0420 | 0.0032 | 0.87 |
| $\beta_3$ | 2 | 0.0694 | 0.0582 | 0.0080 | 0.76 |
| $\sigma_y$ | 1.41 | 0.1968 | 0.3829 | 0.1505 | 0.91 |
| $\log(\lambda_y)$ | 1.10 | -0.6413 | 0.9288 | 0.7867 | 0.99 |
| $\tau_y$ | 1 | -0.0255 | 0.0595 | 0.0048 | 0.91 |

Table S3: Posterior estimates of parameters under models $M_2^{real}$, $M_3^{real}$, and $M_4^{real}$

| | $M_2^{real}$ | | | $M_3^{real}$ | | |
|---|---|---|---|---|---|---|
| Parameters | Mean | SD | 95% HPD interval | Mean | SD | 95% HPD interval |
| $\beta_0$ | 6.9386 | 0.0986 | (6.7465, 7.1313) | 6.9050 | 0.0987 | (6.7126, 7.0997) |
| $\beta_1$ | 0.0023 | 0.0134 | (-0.0255, 0.0266) | 0.0053 | 0.0135 | (-0.0216, 0.0315) |
| $\beta_2$ | 0.2270 | 0.0095 | (0.2084, 0.2456) | 0.3283 | 0.0096 | (0.3093, 0.3470) |
| $\beta_3$ | 0.1632 | 0.0447 | (0.0727, 0.2530) | 0.1664 | 0.0407 | (0.0866, 0.2513) |
| $\beta_4$ | 0.1661 | 0.0136 | (0.1399, 0.1924) | 0.1687 | 0.0137 | (0.1417, 0.1954) |
| $\beta_5$ | 0.2933 | 0.0250 | (0.2442, 0.3437) | 0.2970 | 0.0249 | (0.2478, 0.3463) |
| $\beta_6$ | 0.1475 | 0.0082 | (0.1316, 0.1637) | 0.1481 | 0.0083 | (0.1320, 0.1642) |
| $\tau_y$ | 2.0899 | 0.0638 | (1.8657, 2.2185) | 2.1744 | 0.0627 | (2.0554, 2.2978) |
| $\log(\lambda_y)$ | -0.0948 | 0.9044 | (-1.9761, 1.5107) | -0.1038 | 0.9026 | (-2.0513, 1.4454) |
| $\sigma_y$ | 0.0448 | 0.0415 | (0.0096, 0.0468) | 0.1197 | 0.0392 | (0.0707, 0.2237) |

| | $M_4^{real}$ | | |
|---|---|---|---|
| Parameters | Mean | SD | 95% HPD interval |
| $\beta_0$ | 6.9340 | 0.1045 | (6.7350, 7.1413) |
| $\beta_1$ | 0.0010 | 0.0135 | (-0.0255, 0.0279) |
| $\beta_2$ | 0.2275 | 0.0097 | (0.2081, 0.2460) |
| $\beta_3$ | 0.1622 | 0.0519 | (0.0606, 0.2605) |
| $\beta_4$ | 0.1663 | 0.0138 | (0.1391, 0.1931) |
| $\beta_5$ | 0.2941 | 0.0255 | (0.2445, 0.3440) |
| $\beta_6$ | 0.1482 | 0.0084 | (0.1321, 0.1648) |
| $\tau_y$ | 2.4894 | 0.0645 | (2.3588, 2.6164) |
| $\log(\lambda_y)$ | -0.1314 | 0.8756 | (-1.9592, 1.4213) |
| $\sigma_y$ | 0.1514 | 0.0470 | (0.0818, 0.2717) |

Table S4: Posterior estimates under model $M_1^{real}$ with the CAR structure in the real data analysis

| Parameter | Mean | SD | 95% HPD interval | Parameter | Mean | SD | 95% HPD interval |
|---|---|---|---|---|---|---|---|
| $\beta_0$ | 6.8964 | 0.0935 | (6.7016, 7.0733) | $\alpha_{20}$ | 8.2925 | 0.1405 | (8.0118, 8.5531) |
| $\beta_1$ | 0.0083 | 0.0135 | ( -0.0178, 0.0355) | $\alpha_{21}$ | 0.1945 | 0.0304 | (0.1332, 0.2539) |
| $\beta_2$ | 0.3266 | 0.0096 | (0.3075, 0.3461) | $\alpha_{22}$ | 0.2607 | 0.1213 | (0.0634, 0.5608) |
| $\beta_3$ | 0.1590 | 0.0436 | (0.0629, 0.2389) | $\alpha_{23}$ | -0.6906 | 0.0264 | (-0.7418, -0.6387) |
| $\beta_4$ | 0.1643 | 0.0137 | (0.1383, 0.1917) | $\alpha_{24}$ | 0.3906 | 0.0509 | (0.2883, 0.4887) |
| $\beta_5$ | 0.3010 | 0.0247 | (0.2533, 0.3500) | $\tau_{x2}$ | 0.6731 | 0.0198 | (0.6345, 0.7119) |
| $\beta_6$ | 0.1490 | 0.0081 | (0.1383, 0.1917) | $\sigma_{x2}$ | 0.3163 | 0.1596 | (0.1364, 0.8038) |
| $\tau_y$ | 2.4776 | 0.0628 | (2.3554, 2.5993) | $\phi_2$ | 0.0137 | 0.1937 | (-0.4024, 0.3028) |
| $\sigma_y$ | 0.1375 | 0.0370 | (0.0842, 0.2253) | $\alpha_{10}$ | 3.2307 | 0.1637 | (2.9351, 3.6430) |
| $\phi_y$ | -0.0553 | 0.2073 | (-0.4397, 0.2966) | $\alpha_{11}$ | 0.1025 | 0.1497 | (-0.2225, 0.4408) |
| $\alpha_{12}$ | -0.1267 | 0.0238 | (-0.1724, -0.0804) | $\tau_{x1}$ | 0.9322 | 0.0239 | (0.8867, 0.9792) |
| $\alpha_{13}$ | 0.4921 | 0.0453 | (0.4044, 0.5793) | $\phi_1$ | 0.0083 | 0.2059 | (-0.4178, 0.3119) |
| $\alpha_{14}$ | -0.0209 | 0.0147 | (-0.4096, 0.0083) | $\sigma_{x1}$ | 0.3889 | 0.0889 | (0.2503, 0.5914) |

Table S5: Posterior estimates under the model with the same response and missing covariates models as $M_1^{real}$ but with the missing mechanism model $M_R^{m_2}$

| Parameters | Mean | SD | 95% HPD interval | Parameters | Mean | SD | 95% HPD interval |
|---|---|---|---|---|---|---|---|
| $\beta_0$ | 6.8984 | 0.103 | (6.6918,7.1041) | $\alpha_{20}$ | 8.3053 | 0.1545 | (8.0074,8.624) |
| $\beta_1$ | 0.0073 | 0.0134 | (-0.019,0.0333) | $\alpha_{21}$ | 0.1971 | 0.0297 | (0.1385,0.2559) |
| $\beta_1$ | 0.3274 | 0.0098 | (0.3089,0.3468) | $\alpha_{22}$ | 0.2784 | 0.0901 | (0.1079,0.4706) |
| $\beta_3$ | 0.1602 | 0.0456 | (0.0645,0.2515) | $\alpha_{23}$ | -0.6922 | 0.027 | (-0.7459,-0.64) |
| $\beta_4$ | 0.1655 | 0.0138 | (0.1388,0.1927) | $\alpha_{24}$ | 0.3887 | 0.0508 | (0.2904,0.4874) |
| $\beta_5$ | 0.3011 | 0.025 | (0.2521,0.3499) | $\tau_{x2}$ | 0.6758 | 0.0196 | (0.638,0.7146) |
| $\beta_6$ | 0.1491 | 0.0082 | (0.133,0.1652) | $\log(\lambda_{x_2})$ | 0.6377 | 1.3126 | (-1.7918,3.2036) |
| $\tau_y$ | 2.4755 | 0.0637 | (2.3538,2.6005) | $\sigma_{x_2}$ | 0.3197 | 0.1386 | (0.1484,0.7011) |
| $\log(\lambda_y)$ | -0.0616 | 0.9111 | (-1.9507,1.5688) | $\alpha_{10}$ | 3.0889 | 0.1836 | (2.6708,3.4172) |
| $\sigma_y$ | 0.1408 | 0.0524 | (0.0705,0.2807) | $\alpha_{11}$ | 0.0628 | 0.1401 | (-0.203,0.3587) |
| $\alpha_{12}$ | -0.1256 | 0.0238 | (-0.173,-0.0801) | $\alpha_{13}$ | 0.4922 | 0.045 | (0.4039,0.5798) |
| $\alpha_{14}$ | -0.0195 | 0.0147 | (-0.0484,0.0096) | $\tau_{x_1}$ | 0.9313 | 0.0238 | (0.886,0.9773) |
| $\log(\lambda_{x_1})$ | 0.6211 | 1.2485 | (-1.7725,2.9121) | $\sigma_{x_1}$ | 0.4373 | 0.1436 | (0.2416,0.7792) |

Table S6: Posterior estimates of missingness mechanism models $M_R^{m_2}$ with different response and missing covariates models

| Parameters | Mean | SD | 95% HPD interval | Parameters | Mean | SD | 95% HPD interval |
|---|---|---|---|---|---|---|---|
| $M_1^{real}$ (mDIC = 8966.80 and DIC($R$) = 7963.12) | | | | | | | |
| $\phi_{10}$ | -4.6259 | 0.6950 | (-6.0544, -3.3289) | $\phi_{20}$ | 4.2463 | 0.5596 | (3.1820, 5.3536) |
| $\phi_{11}$ | 0.2636 | 0.2946 | (-0.2867, 0.8782) | $\phi_{21}$ | 0.0323 | 0.1903 | (-0.3315, 0.4290) |
| $\phi_{12}$ | 2.1588 | 0.0768 | (2.0105, 2.3105) | $\phi_{22}$ | 0.8638 | 0.0389 | (0.7889, 0.9393) |
| $\phi_{13}$ | 2.0937 | 0.1140 | (1.8730, 2.3161) | $\phi_{23}$ | -0.1072 | 0.0781 | (-0.2621, 0.0436) |
| $\phi_{14}$ | -0.1665 | 0.0383 | (-0.2421, -0.0925) | $\phi_{24}$ | 0.0753 | 0.0268 | (0.0231, 0.1276) |
| $\phi_{15}$ | 0.2179 | 0.2832 | (0.1120, 0.3421) | $\phi_{25}$ | -0.4423 | 0.0473 | (-0.5335, -0.3484) |
| $\phi_{16}$ | 0.5952 | 0.2944 | (0.2243, 1.3737) | $\phi_{26}$ | 0.6846 | 0.2904 | (0.3300, 1.4627) |
| $\phi_{17}$ | 0.7491 | 0.2832 | (0.3493, 1.4431) | $\phi_{27}$ | 0.0348 | 0.1324 | (-0.2120, 0.3207) |
| $M_2^{real}$ (mDIC = 8979.23 and DIC($R$) = 7965.87) | | | | | | | |
| $\phi_{10}$ | -4.8978 | 0.7743 | (-6.3297,-3.3795) | $\phi_{20}$ | 4.2702 | 0.5568 | (3.2429,5.4549) |
| $\phi_{11}$ | 0.2152 | 0.2220 | (-0.2266,0.6593) | $\phi_{21}$ | 0.0425 | 0.1862 | (-0.3485,0.4195) |
| $\phi_{12}$ | 2.2037 | 0.0789 | (2.0504,2.3577) | $\phi_{22}$ | 0.8723 | 0.0397 | (0.7953,0.9497) |
| $\phi_{13}$ | 2.1295 | 0.1183 | (1.9015,2.3584) | $\phi_{23}$ | -0.1331 | 0.0802 | (-0.2861,0.0250) |
| $\phi_{14}$ | -0.1507 | 0.0387 | (-0.2256,-0.0750) | $\phi_{24}$ | 0.0732 | 0.0274 | (0.0187,0.1265) |
| $\phi_{15}$ | 0.2461 | 0.0657 | (0.1178,0.3747) | $\phi_{25}$ | -0.4407 | 0.0485 | (-0.5343,-0.3462) |
| $\phi_{16}$ | 0.0840 | 0.5196 | (-0.8713,0.9425) | $\phi_{26}$ | 0.1868 | 0.3976 | (-0.6105,0.8710) |
| $\phi_{17}$ | 0.2240 | 0.4956 | (-0.7861,1.1051) | $\phi_{27}$ | -0.0031 | 0.4097 | (-0.7750,0.7150) |
| $M_3^{real}$ (mDIC = 8970.98 and DIC($R$) = 7963.98) | | | | | | | |
| $\phi_{10}$ | -4.9853 | 0.7242 | (-6.4871,-3.6718) | $\phi_{20}$ | 4.2382 | 0.6101 | (3.0024,5.4249) |
| $\phi_{11}$ | 0.1926 | 0.2547 | (-0.3255,0.7045) | $\phi_{21}$ | 0.0258 | 0.1884 | (-0.3371,0.4144) |
| $\phi_{12}$ | 2.2104 | 0.0792 | (2.0590,2.3683) | $\phi_{22}$ | 0.8591 | 0.0393 | (0.7833,0.9371) |
| $\phi_{13}$ | 2.1171 | 0.1191 | (1.8838,2.3470) | $\phi_{23}$ | -0.1167 | 0.0798 | (-0.2757,0.0370) |
| $\phi_{14}$ | -0.1509 | 0.0383 | (-0.2247,-0.0757) | $\phi_{24}$ | 0.0705 | 0.0270 | (0.0172,0.1242) |
| $\phi_{15}$ | 0.2514 | 0.0646 | (0.1298,0.382) | $\phi_{25}$ | -0.4426 | 0.0514 | (-0.5429,-0.3398) |
| $\phi_{16}$ | 0.0105 | 0.4008 | (-0.8457,0.8195) | $\phi_{26}$ | 0.5740 | 0.2357 | (0.2294,1.1566) |
| $\phi_{17}$ | -0.6727 | 0.2349 | (-1.2782,-0.3669) | $\phi_{27}$ | -0.2105 | 0.1186 | (-0.4898,-0.0185) |
| $M_4^{real}$ (mDIC = 8969.02 and DIC($R$) = 7963.75) | | | | | | | |
| $\phi_{10}$ | -5.1101 | 0.8917 | (-7.3005,-3.6607) | $\phi_{20}$ | 4.1047 | 0.6179 | (2.9729,5.5808) |
| $\phi_{11}$ | 0.2995 | 0.3292 | (-0.2149,1.2075) | $\phi_{21}$ | -0.0048 | 0.2183 | (-0.4737,0.4456) |
| $\phi_{12}$ | 2.1847 | 0.0776 | (2.0358,2.3391) | $\phi_{22}$ | 0.8749 | 0.0387 | (0.7993,0.9500) |
| $\phi_{13}$ | 2.0873 | 0.1148 | (1.8669,2.3138) | $\phi_{23}$ | -0.1237 | 0.078 | (-0.2762,0.0295) |
| $\phi_{14}$ | -0.1603 | 0.0386 | (-0.2365,-0.0857) | $\phi_{24}$ | 0.0736 | 0.027 | (0.0216,0.1272) |
| $\phi_{15}$ | 0.2389 | 0.0623 | (0.1211,0.3636) | $\phi_{25}$ | -0.4177 | 0.0471 | (-0.5124,-0.3277) |
| $\phi_{16}$ | 0.5403 | 0.1977 | (0.2640,1.0230) | $\phi_{26}$ | 0.4815 | 0.1719 | (0.2516,0.9297) |
| $\phi_{17}$ | 0.6820 | 0.6404 | (-0.1046,2.5732) | $\phi_{27}$ | -0.2497 | 0.4021 | (-1.1857,0.6954) |
